# Supplementary material for: SplitMeanFlow: Interval Splitting Consistency in Few-Step Generative Modeling
Source: arXiv:2507.16884 source file (2025-07-22)
Supplement: Supplementary file 1 [file appendix.tex]

\section{Hello World}
%\subsection{Hello World}
